# Supplementary material for: Type II multiferroic order in two-dimensional transition metal halides from first principles spin-spiral calculations
Source: arXiv:2301.05107 source file (2023-01-12)
Supplement: Supplementary file 1 [file supp.tex]

%
% ****** End of file apssamp.tex ******
